# Supplementary material for: Analyzing Data-Centric Properties for Graph Contrastive Learning
Source: arXiv:2208.02810 source file (2023-01-23)
Supplement: Supplementary file 1 [file datacentric_properties.tex]

\textcolor{blue}{As discussed in Sec. \ref{sec:preliminaries}, many analyses of self-supervised representation learning assume, either implicitly\cite{Zimmermann_Inverts,Huang_sslgen21} or explicitly\cite{HaoChen_SpectralCL,Wei21_SelfTraining,Balcan04}, that there exists a latent space that is \emph{invariant} to augmentation functions and supports the properties of \emph{recoverability} and \emph{separation}. In Fig. \ref{fig:data_props}, we illustrate these properties via the aid of a figure.}
